# Supplementary material for: Parametric Graph Templates: Properties and Algorithms
Source: arXiv:2011.07001 source file (2020-11-13)
Supplement: Supplementary file 1 [file sec-si.tex]

\subsubsection{Subgraph Isomorphism}

Our algorithm is a generalization of an FPT subgraph isomorphism algorithm~\cite{EPPSTEIN}. We describe its most important aspects here, and then discuss the changes and all the details necessary for our more general case  in \Cref{sec:autotemplate:dec}. Note that interestingly, in instance isomorphism we are ultimately trying to answer if two graphs are isomorphic, but we reduce the problem to matching only subgraphs that are chosen in a way that connects the tree decomposition and the template hierarchy.

In subgraph isomorphism, we consider a pattern graph $G'$ and a target graph $G$ and we want to decide if there is a subgraph of $G$ that is isomorphic to $G'$.

The idea for subgraph isomorphism is to do a kind of dynamic programming on the decomposition tree, where at every node we record all the possible ways the subgraph induced by the node maps to the pattern graph. Moreover, the state keeps track of which vertices in the pattern have already been matched in a child node, and which vertices in the pattern have not yet been matched.

A \emph{partial match} $(\phi, U, C)$ at node $A$ contains:
\begin{itemize}
\item The set of \emph{unmatched vertices} $U$, which is a subset of the pattern's vertices. It should contain vertices that have not been matched in $A$ or any of its descendants.
\item The set of \emph{vertices matched in a child} $C$, which is a subset of the pattern's vertices. This set should contain the vertices that were mapped in a child node of $A$, but that are not in $A$ itself.
\item A function $\phi$ from the vertices in the pattern that are neither in $U$ nor in $C$ to the vertices in $A$. This function establishes the isomorphism between a subgraph of the pattern and the subgraph of the graph induced by $A$. If the subgraph isomorphism works out, then it will be possible to "piece together" suitable $\phi$ functions to create the function that establishes the subgraph isomorphism.
\end{itemize}
One can come up with rules on how to combine partial matches of the children into partial matches of a parent node that match the intuitive meaning of the partial matches, such that if we find a partial match of the root node where the set of unmatched vertices $U$ is empty, then there is a subgraph isomorphism between the pattern and the target graph.

For example, if a vertex is unmatched in a parent, it has to be unmatched in the child as well. Moreover, if a vertex is matched in a child at a node, then it has to be matched in a child at its parent too. Another rule is that if a vertex is matched in a child, it has to be unmatched in exactly one of the two children. We will not list all the rules necessary for subgraph isomorphism, as we will discuss the detailed more general rules for our case in \Cref{sec:autotemplate:dec}.

\subsection{Deciding Instance Isomorphism}\label{sec:autotemplate:dec}

Similarly to template discovery, we will focus our attention on target graphs with bounded treewidth $\tau$. The naive way to decide instance isomorphism is to instantiate the template and check if the graphs are isomorphic. This takes $2^{O(\tau^5 \log \tau)}n'^5$ time~\cite{DBLP:conf/focs/LokshtanovPPS14}. We improve the dependence on the size $n'$ of the target graph to quadratic in $n'$, at the cost of increasing the dependence on the size $n$ of the template.

%Our goal is to find an algorithm that has a small runtime in terms of $n$, but is allowed to have a large runtime in $n'$, $m'$, and the treewidth.In our case, our parameters are $m$ and a structural parameter of the graph $G'$ (called treewidth). We want a runtime that is polynomial in $N+M$ and can grow as any function of $\theta$.

The algorithm has a \emph{filtering phase for each template}. The phases are run for the templates in the post-order of the template tree. Each phases filters a set of possible states in a dynamic program, until only states remain that agree with all templates. We first discuss the dynamic program without this filtering. This dynamic program fails because it cannot ensure that every template $T_i$ is instantiated $P_i$ times, in fact it completely disregard the number of instances that are made (and can even have different number of instances for the same template). We will explain the filtering at the end of the section.

\subsubsection{Unfiltered Basic DP}

For simplicity, let us start with the special case where the decomposition tree is a path $\mathcal{A}$. We then show how to extend the algorithm to the binary tree case in \Cref{sec:autotemplate:general}.
%The goal is to get a dynamic programming solution in a similar way as we sketched for subgraph isomorphism. %$% (which we assume to be a path, for now).
%
%First: Simpler Case of Pathwidth Decomposition.

At any node $A_i$ encountered when walking up the path $\mathcal{A}$, we want to maintain a \emph{partial match} between the subgraph of $G'$ induced by the vertices in the subtree rooted at $A_i$ and the template graph. To keep the state space small, we only maintain the matches explicitly for the vertices in $A_i$. For the rest of the vertices that we already matched, we must find a compact representation that still allows us to extend the partial match. 

This representation must enable us to ensure two key properties (that together imply the isomorphism through providing a suitable bijection) -- There are parameters $\mathcal{P}$ such that the instantiation of $(G, \mathcal{T}, \mathcal{P})$ satisfies:
\begin{enumerate}
	\item Every vertex in the graph $G'$ is matched to at most one vertex in the instantiation (No Ambiguity).
	\item In every instance, all the vertices in the instance are matched with a vertex in $G'$ (No Incomplete Instances).
\end{enumerate}
Keeping track of all the already matched vertices is infeasible, as that would create a state space exponential in $n'$. Thus, we only keep information for a subset of the instances (called \emph{active instances}), which we define below. This is the main difference to the subgraph isomorphism algorithm.
%We cannot afford to keep track of all vertices that we already matched (not even a single bit for each of them) because that would create a state space exponential in $n'$. The idea is that we keep this information only for certain "important instances".

Instances here take on the role of combinatorial entities in the matching algorithm. %If the matching algorithm succeeds, they correspond to instances of a parametric graph $(G, \mathcal{T}, \mathcal{P})$ for some set of parameters $\mathcal{P}$ not known a priori.
Specifically, the algorithm maintains, at each node in the decomposition, a subtree of an instance hierarchy (that corresponds to the templates $\mathcal{T}$ we want to match).

Next, we define which instances we need to keep track of. An instance $I_j$ of a template is \emph{active} at node $A$ if $A$ contains a vertex that is in $I_j$ (i.e. a vertex that belongs to $I_j$ or one of its descendants). An instance that is not active is called \emph{inactive}.

The key observation is that we only need to keep track of the $O(h\tau)$ \emph{active instances}, for which we store which vertices we already matched. The idea for the algorithm is that when an instance becomes inactive at $A$, then all its vertices must be matched in a descendant of $A$. In \Cref{lem:autotemplate-active}, we show that once an instance becomes inactive, it never becomes active again (i.e., it is safe to "forget about" such an instance).

Formally, a partial match $(\phi, U, C, \mathcal{I}, F)$ at node $A$ consists of: 
\begin{itemize}
	\item A subtree $\mathcal{I}$ of an instance tree (each instance corresponds to a template in $\mathcal{T}$). Each node in this instance tree is either active or is a leaf node in the subtree $\mathcal{I}$. An active instance has one inactive leaf node for each child template that does not have an active instance.
	\item The set of \emph{unmatched vertices} $U$ contains a set of vertices of the active instances.
	\item The set of \emph{vertices matched in a child} $C$ contain vertices of the active instances.
	\item The function $\phi$ is a mapping from the vertices of $A$ to the vertices in the active instances of $\mathcal{I}$. Specifically, every non-leaf node of $\mathcal{I}$ must contain at least one vertex matched by~$\phi$.
	\item The set of \emph{fully matched instances} $F$ contains inactive instances of $\mathcal{I}$. If an inactive instance is in the set $F$, this means that we already matched at least one instance of the corresponding template.
\end{itemize}

Any partial match must ensure that the induced subgraphs that are matched by the mapping $\phi$ are isomorphic. Moreover, $U$ and $C$ must be disjoint and any vertex in $A$ must be either matched by $\phi$, be in $U$, or in $C$.

The algorithm can be specified by providing the state space and the rules for extending a partial match of a child node $A$ of $\mathcal{A}$ to a partial match of the parent node $A'$ of $A$. If the algorithm constructs a partial match  $( \phi, U, C, \mathcal{I}, F)$ of the root of $\mathcal{A}$ where $U$ is empty and $F$ contains all non-active instances of $I$, then the algorithm returns true (the graph $G'$ is an instance of the templates) otherwise it returns false.

Consider a partial match $( \phi, U, C, \mathcal{I}, F)$ of $A$ and a candidate partial match $( \phi_p, U_p, C_p, \mathcal{I}_p, F_p)$ of the parent $A_p$ of $A$. The following conditions must hold to validate the parent's partial match:

\begin{enumerate}
	\item The matchings $\phi$ and $\phi_p$ agree on the vertices that are both in $A$ and $A_p$.
	\item For all vertices $v$ that are in an active instance of $\mathcal{I}_o$:
	\begin{enumerate}
	\item If $v$ is matched by $\phi$, but is not in $A$, it is in $C_p$.
	\item If $v$ in in $C$, it is also in $C_p$
	\item If $v$ is in $U_p$ and in an active instance of $\mathcal{I}$, it is also in $U$.
	\end{enumerate}
	\item If an instance is active in $\mathcal{I}$ and becomes inactive in $\mathcal{I}_p$ (or does not appear in $\mathcal{I}_p$ at all), then: 
	\begin{enumerate}
	\item All its inactive children are fully matched (i.e., in $F$) 
	\item No vertex that belongs to the instance is unmatched (i.e., in $U$).
	\item If this instance does appear in $\mathcal{I}_p$, then it is in $F_p$.
	\end{enumerate}

\end{enumerate}
Notice that conditions $(1)$ and $(2)$ are adapted from the subgraph isomorphism algorithm by adding the constraint that we only keep track of vertices in the active instances. Conditions $(1)$ and $(2)$ ensure that there is no ambiguity and adding Condition $(3)$ ensures that there are no incomplete instances.

The next lemma ensures that it is always well-defined how the instances in the instance tree of the parent relate to those in the child.
\begin{lemma}
	If an instance is active at a node $A$ and its child $A'$, then there is a vertex in $A\cap A'$ that is mapped to the instance.
\end{lemma}
\begin{proof}
	Consider otherwise. Consider the subgraph $G''$ of the instance induced by the vertices that are in $A'$ and its descendants, and the subgraph $G'$ of the instance induced by the vertices that are in $A$ and its ancestors. Because the instance is connected, there must be an edge from $G'$ to $G''$. By definition of the tree decomposition, there must be a node that contains both endpoints. But this contradicts our assumption that $A\cap A'$ does not contain any vertices of the instance.
\end{proof}

The next lemma proves the correctness of Condition (3). It means that there is no way that when an instance becomes inactive, but has not yet been fully matched, it could becomes completed / fully matched at some ancestor in the tree decomposition. 
\begin{lemma}\label{lem:autotemplate-active}
	If an instance of $T$ is active at a child of $A$ and is inactive at $A$, the instance will stay inactive at all ancestors of $A$.
\end{lemma}
\begin{proof}
	Consider otherwise. Consider the first node $\tilde A$ along the way to the root of $\mathcal{A}$ where the instance is active again. This node $\tilde A$ thus contains a vertex $u$ that is in $T$.
	
	\emph{Case 1: $T$ contains only the vertex $u$.} Then, because the instance was active in a child of $A$, the child of $A$ must contain $u$. But this contradicts that all vertices occur in contiguous subtrees of $\mathcal{A}$ ($u$ is in a child of $A$, in an ancestor of $A$, but not in $A$).
	
	\emph{Case 2: $T$ contains at least one other vertex. }%There might be other vertices in $\tilde A$ that are in $T$. Let $U$ contain the set of these vertices.
	Because the instance was active in a child of $\tilde A$, there is a vertex $v$ in this child of $\tilde A$ that is in $T$. If the vertex $u$ is the only such vertex, finish the case in the same way as Case 1. Otherwise, consider the path from $u$ to $v$ that only uses vertices in $T$ (such a path exists because the subgraph induced by a template is connected). Some of the vertices along this path occur in the node $\tilde A$, and some occur in a descendant of $A$. Consider the first edge $(u', v')$ going from a node that occurs in $\tilde A$ to a node that occurs in the child of $A$. By definition of the tree decomposition, there must be a node that contains both $u'$ and $v'$. This node cannot be $A$ because it does not contain either vertex (otherwise the instance would be active at $A$). If this node is in a descendant of $A$, then $u'$ is not in a contiguous subtree of the decomposition tree (contradicting the definition of a tree decomposition). Similarly, if this node is in an ancestor of $A$, then $v'$ would not be in a contiguous subtree.
\end{proof}
Observe that if we would consider an instance to be active only when a vertex that belongs to it is in the node, then the proof would fail, because we cannot necessarily find a vertex that is in $T$ and not in $A$.

\begin{lemma}\label{lem:autotemplate:combinatorics}
	There are $2^{O(h \tau \log \tau + \tau \log (\tau n) )}$ partial matches at every node $A$ in the tree decomposition.
\end{lemma}
\begin{proof}
There are $3^{\tau}$ choices for how to distribute the vertices in $A$ between $C$, $U$, and those that are matched by $\phi$.

There are at most $h\tau + n$ instances in the instance tree $I$, containing at most $\tau n$ vertices. Hence, there are at most $(\tau n)^\tau$ possibilities to match those vertices to the vertices in $A$.

To enumerate all possible trees $I$, pick the $\tau$ templates of the active instances first. Then, choose the instance numbers for the templates one after the other. This leads to at most $\tau(\tau!)^h$ choices overall.

\end{proof}
%This gives an overall runtime of $2^{O(h \tau \log \tau + \tau \log (\tau n) )}O(M)$.

\subsubsection{Filtering} \label{sec:autotemplate:filter}

We extend the state space by counting the number of inactive (already fully matched) instances, but \emph{only for one template $T_i$ at a time}. This number can easily be maintained by counting how many instances of this template become inactive. The additional rule is that once the parent of an instance of $T_i$ becomes inactive, then $P_i$ instances must have been fully matched. 

We iterate this filtering on the "basic" state space from the basic DP until all templates have been filtered. The templates are filtered in their post-order traversal of the template tree. The algorithm checks in the end if a partial match of the root of $\mathcal{A}$ with no unmatched vertices remains.

The state space increase by a factor of $P_i$ in the filtering of $T_i$. Because we filter one template after the other, the overall runtime increases by a factor $O(\sum_i P_i)$. Because template graphs are nonempty, $\sum_i P_i \in O(n')$ (Increasing a parameter also increases the size of the instance at least as much).

%This gives an overall runtime of $2^{O(h \tau \log \tau + \tau \log (\tau n) )}O(m'n')$.

\subsubsection{Extension to Tree Decompositions}\label{sec:autotemplate:general}

To extend the approach to trees we need to specify an additional rule what partial matches of two children nodes need to satisfy to be \emph{compatible} with the parent's partial match.
The additional rule, which ensures that we do not have any collisions is that: Consider a parent $A_p$ with children $A_l$ and $A_r$.
For every vertex $v$ in an instance that is active in the parent and both of its children:
\begin{itemize}
	\item If the vertex $v$ is marked as \emph{matched in a child} at the parent $A_p$, it is unmatched in exactly one of the two children nodes.
\end{itemize}

\begin{theorem}
On a connected target graph of treewidth $\tau$ with $n'$ edges and a connected template graph with $n$ vertices and a template tree of height $h$, instance isomorphism takes $2^{O(h \tau \log \tau + \tau \log (\tau n) )}m'n'$ time. \end{theorem}
\begin{proof}
By \Cref{lem:autotemplate:combinatorics}, there are $2^{O(h \tau \log \tau + \tau \log (\tau n) )}$ partial matches at every node of the decomposition. At each of the $O(m')$ nodes in the decomposition tree, we need to consider all possible combinations of partial matches for a parent and its (at most) two children, which is in $2^{O(h \tau \log \tau + \tau \log (\tau n) )}m'$. The overhead for the filtering is $O(n')$ as discussed in \Cref{sec:autotemplate:filter}.
\end{proof}

%\subsection{Constructing Instance Isomorphisms}

%To construct the parameters for an instance isomorphism, we can think of a hypergraph of partial matches: The vertices are the partial matches, and there is a hyperedge between a parent node's partial match and two of its children's partial matches if the two partial matches are compatible with the parent's partial match.

%Start from the root node and pick some hyperedge. Continue the search for both children node's partial matches. This search creates a tree of partial matches. In this tree, we can count how many times an instances of a template becomes inactive and 
